# Supplementary material for: Polarimetric Inverse Rendering for Transparent Shapes Reconstruction
Source: arXiv:2208.11836 source file (2022-08-25)

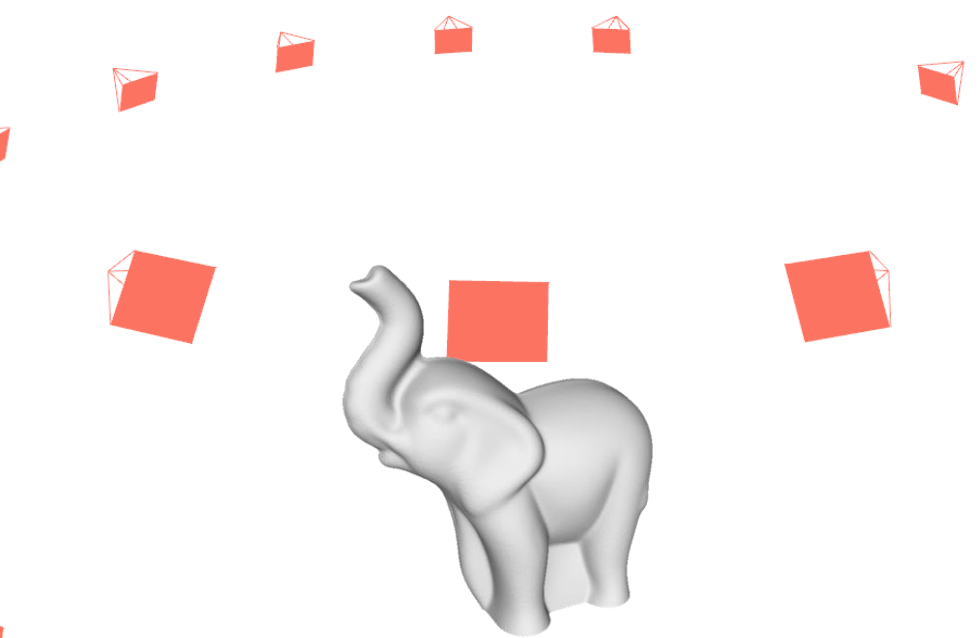

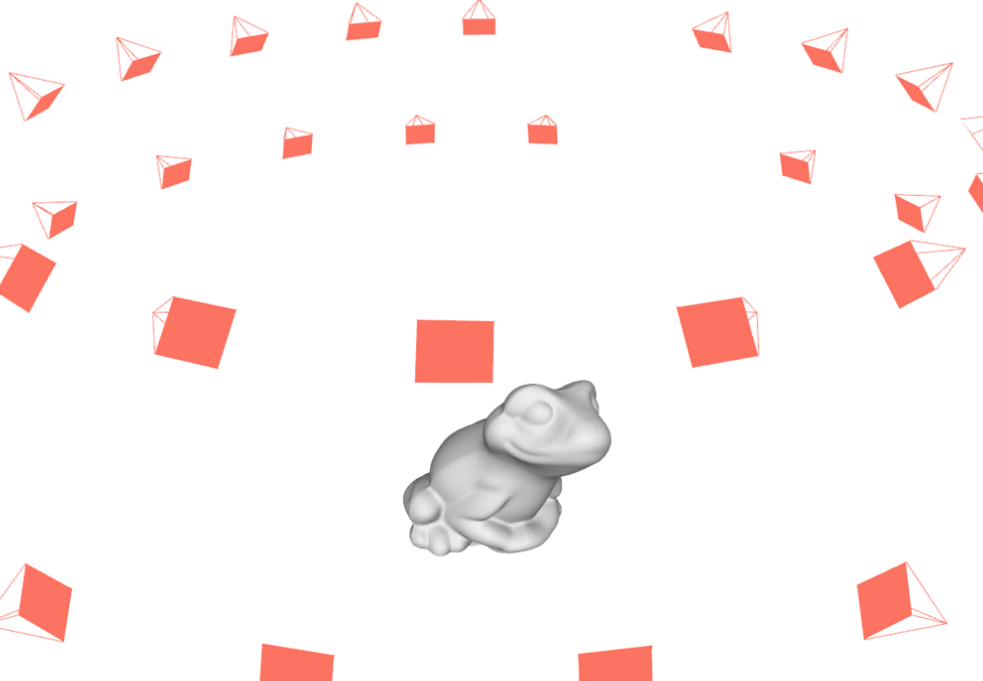

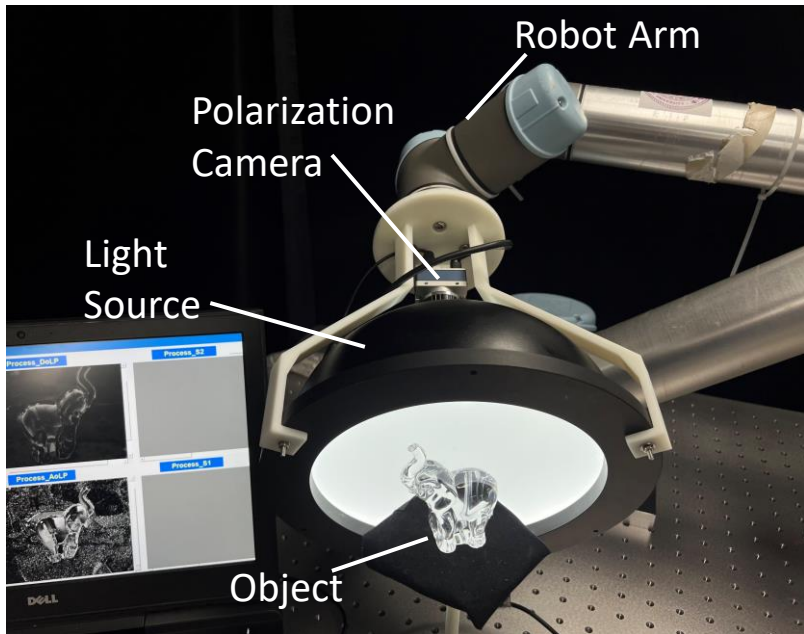

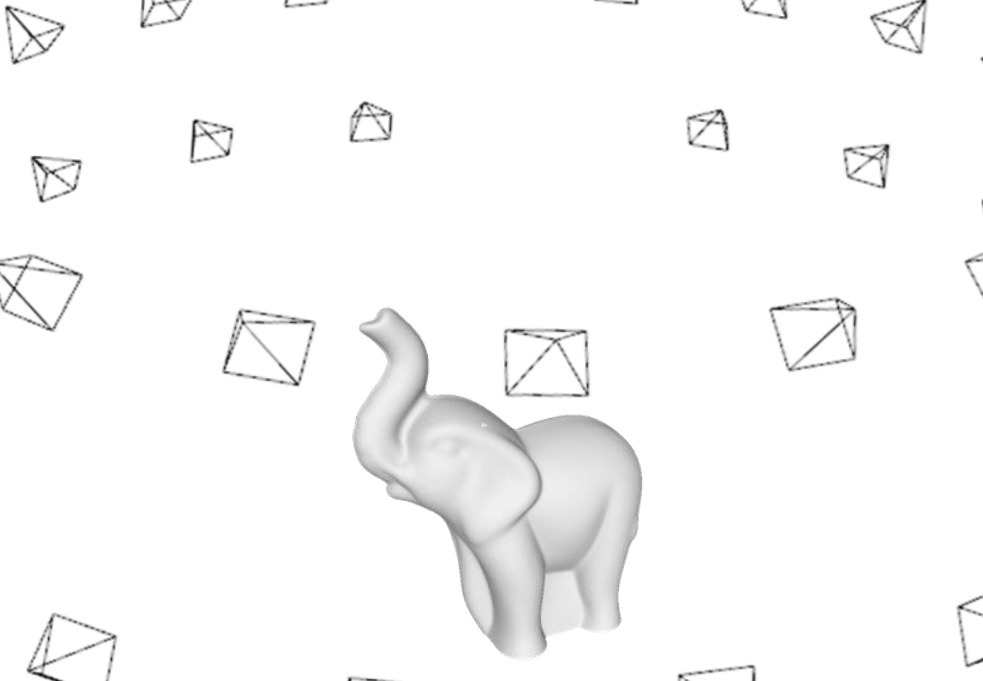

Supplement: Supplementary file 1 [file dataset-supp.pdf]
